# Supplementary material for: Relative Stability and Local Curvature Analysis in Carbon Nanotori
Source: arXiv:1503.04429 source file (2015-03-15)
Supplement: Supplementary file 1 [file torus15-SM.pdf]

# Supplemental on-line material for
# Relative Stability and Local Curvature Analysis in Carbon Nanotori


Chern Chuang,[1] Jie Guan,[2] David Witalka,[2] Zhen Zhu,[2] Bih-Yaw Jin,[3] and David Tománek[2,*]

[1] *Department of Chemistry, Massachusetts Institute of Technology, Cambridge, MA 02139, USA*
[2] *Physics and Astronomy Department, Michigan State University, East Lansing, Michigan 48824, USA*
[3] *Department of Chemistry and Center for Emerging Material and Advanced Devices, National Taiwan University, Taipei 10617, Taiwan*


### Nanotori with different shape parameters

As discussed in the main text, the global and local curvature energy depends sensitively on the shape parameters of polygonal nanotori. The structure, distribution of local Gaussian curvature $G$ and local curvature energy $\Delta E_c/A$ across the surface of all the nanotori presented in Fig. 6 of the main manuscript are displayed in Figs. S1, S2, and S3.

In Fig. S1 we present the series of $D_{6h}$-symmetric polygonal nanotori with changing length $L$ of nanotube segments that were investigated in Fig. 6(b) of the main manuscript. As is discussed in the main text, a $D_{nh}$-symmetric nanotorus can be viewed as $n$ straight CNT segments connected by $n$ elbow joints, the loci of non-hexagonal rings. As the side length $L$ increases, the torus can be asymptotically described by a hexagon of connected nanotubes. On a per-atom basis, the contribution to the excess energy from the elbow joints is negligible in the $L \to \infty$ limit. Thus, the elastic energy is accounted for simply by the summation of the energy of the six constituent CNTs in this limit.

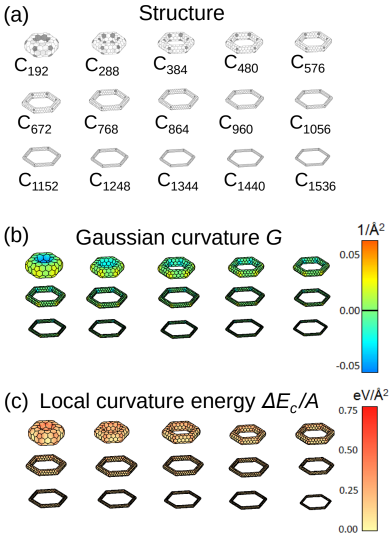


FIG. S1. (Color online)(a) Structural models, (b) local Gaussian curvature $G$ and (c) local curvature energy $\Delta E_c/A$ across the surface of torus isomers with different lengths of the nanotube segments $L$, defined in Fig. 6(a) of the main manuscript. The non-hexagonal rings in (a) are shaded. The values of $G$ and $\Delta E_c/A$ have been interpolated from their values at the atomic sites.

In Fig. S2 we present the series of polygonal nanotori resembling a segment of height $H$ of a double-walled CNT that were investigated in Fig. 6(c) of the main manuscript. The inner and outer tubes are connected at the top and the bottom by lip-lip interactions consisting of hexagonal and non-hexagonal rings. In the $H \to \infty$ limit, the elastic energy contribution from the two ends is a constant, and the nanotorus essentially resembles an infinitely long double-walled CNT in terms of stability.

In Fig. S3 we present polygonal nanotori with changing rotational symmetry number $n$ that were investigated in Fig. 6(d) of the main manuscript. We focus on two families of nanotori and display them in Fig. S3(a-c) and Fig. S3(d-f). In each of the two families, the relative positions of the non-hexagonal rings remain the same while

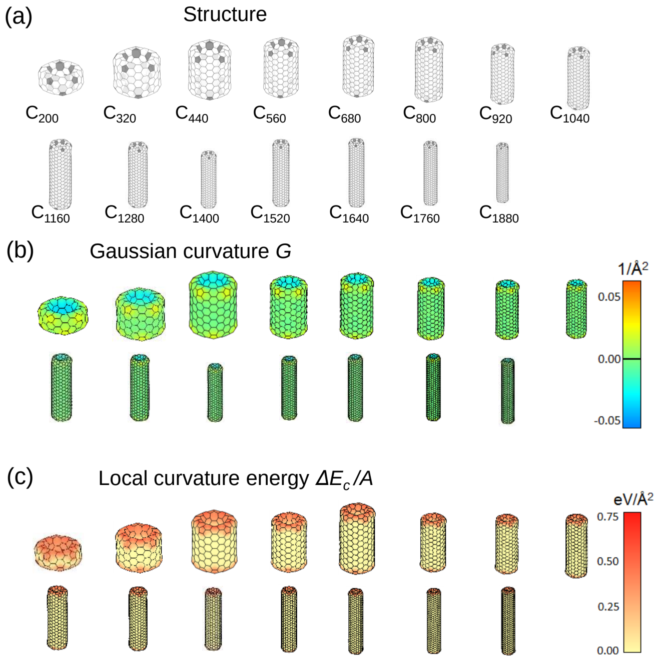


FIG. S2. (Color online)(a) Structural models, (b) local Gaussian curvature $G$ and (c) local curvature energy $\Delta E_c/A$ across the surface of torus isomers with different heights $H$, defined in Fig. 6(a) of the main manuscript. The non-hexagonal rings in (a) are shaded. The values of $G$ and $\Delta E_c/A$ have been interpolated from their values at the atomic sites.

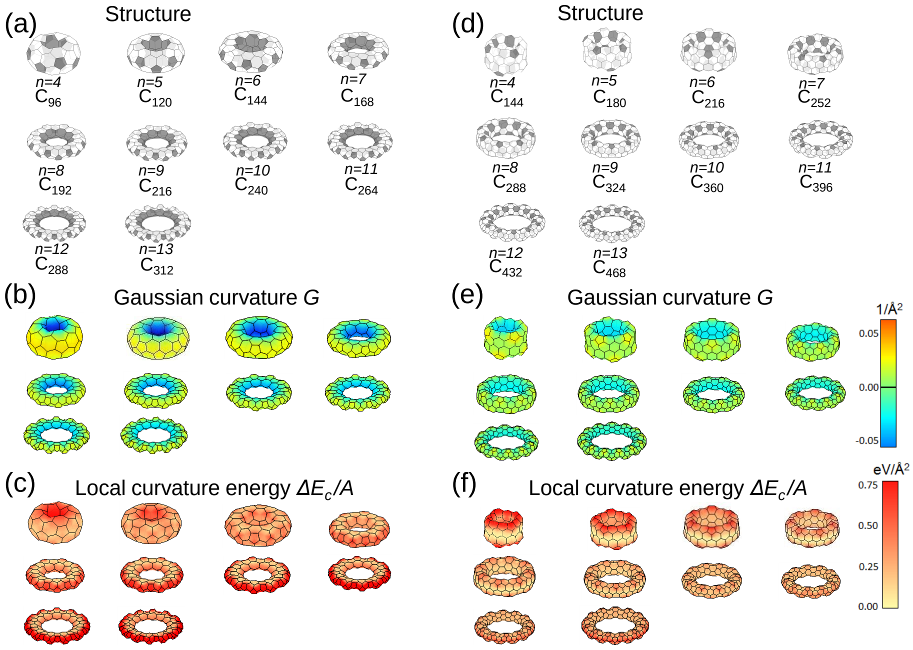


FIG. S3. (Color online)(a,d) Structural models, (b,e) local Gaussian curvature $G$ and (c,f) local curvature energy $\Delta E_c/A$ across the surface of torus isomers with different rotational symmetry numbers $n$, defined in Fig. 6(a) of the main manuscript. Structures in (a-c) and (d-f) represent two distinct torus families. The non-hexagonal rings in (a,d) are shaded. The values of $G$ and $\Delta E_c/A$ have been interpolated from their values at the atomic sites.

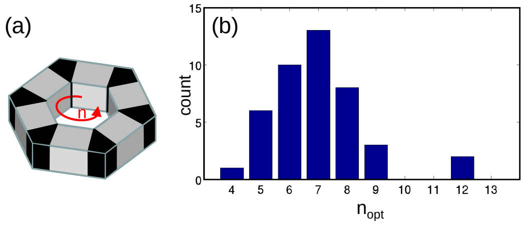


FIG. S4. (Color online)(a) A schematic model of a polygonal nanotorus with an $n$-fold ($n = 6$ in this case) symmetry. (b) Distribution of the optimal rotational symmetry numbers $n_{opt}$ in the 43 families of polygonal nanotori covered in this study.

the rotational symmetry number $n$ changes from $n = 4$ to $n = 13$. Depending on the detailed arrangement of the non-hexagonal rings, we find that the local curvature and strain energy distribution changes strongly. Even more important, the dependence of the strain energy on $n$ is very different for the two families of nanotori, as seen in Fig. 6(d) of the main manuscript.

The change in the distribution of the local curvature in the two families of nanotori is evident when comparing results in Fig. S3(c) and S3(f) for increasing values of $n$. In the first family of nanotori in Fig. S3(c), we observe an abrupt redistribution of the curvature energy from the inner part to the outer part of the torus with increasing $n$. As seen in Fig. S3(f), such a transition does not occur in the second family of nanotori. There, the curvature energy is largest at the top and the bottom rims for small values of $n$ and is gradually redistributed to the outer part for large $n$ values.

To better examine the stability of nanotori as a function of $n$, we selected most stable structures from a huge pool of polygonal nanotori. Our selection criterion was that the heat of formation be less than +0.8 eV/atom based on the AM1 total energy functional[1] and number of atoms per rotational unit cell be at most 40. While AM1 is not as reliable as density functional theory calculations, it provides reasonable energy estimates, including the value of +0.7 eV for the heat of formation of the $C_{60}$, somewhat larger than the observed value of +0.4 eV. The above stated selection criterion filtered out 43 nanotori with different distributions of non-hexagonal rings, defining a torus family. For each of the 43 families, we varied the rotational symmetry number $n$ in the range $4 \leq n \leq 13$ to find the optimal value of $n$. The distribution of the $n_{opt}$ is shown in Fig. S4(b). As mentioned in the main text, the distribution is roughly a Gaussian centered at $n_{opt} = 7$, with some surprising outliers at $n_{opt} = 12$.

* tomanek@pa.msu.edu

[1] M. J. S. Dewar, E. G. Zoebisch, E. F. Healy, and J. J. P. Stewart, J. Am. Chem. Soc. **107**, 3902 (1985).
